# Supplementary material for: Generating Long-term Trajectories Using Deep Hierarchical Networks
Source: arXiv:1706.07138 source file (2017-06-21)
Supplement: Supplementary file 1 [file sec-supplementary.tex]

\section{Supplementary material}
\label{sec:supplementary}

\subsection{Data format and pre-processing}\label{supp:data}

In the temporal domain, the raw tracking data is recorded at 25 Hz. We sub-sampled the possessions in the temporal domain by extracting sequences of 200 frames (= 8 seconds) long at random starting points, using only every 4 frames to reduce the model complexity and redundancy. In this way, we obtained 120.000 training tracks of 50 frames and 20.000 tracks as a holdout set.

In the spatial domain, without loss of generality, we only considered possessions in a half-court of size $50\times 45$ feet. We used a discretized representation of the spatial domain and sampled the raw input tracking data at different spatial resolutions at train-time: this is necessary as the raw tracking data is very sparse in the natural 1-hot occupancy representation using a 1-ft by 1-ft spatial resolution (= $50\times 45 = 2250$ grid cells). For training, we used a resolution of 0.25ft $\times$ 0.25ft (= $400\times380$ cells). We found that dynamically downsampling the input data at multiple resolutions ($400 \times 360$, $200 \times 180$, $50 \times 45$, $25 \times 15$, $10 \times 9$) using max-pooling layers provided enough signal for the model to be trainable.

\begin{figure}[t]
 \centering
 \subcaptionbox{\CORR{optional}Track segmentation and heuristic definition of macro-goals.\label{fig:tracks}}{
  \centering
\includegraphics[width=0.3\textwidth, height=0.33\textwidth]{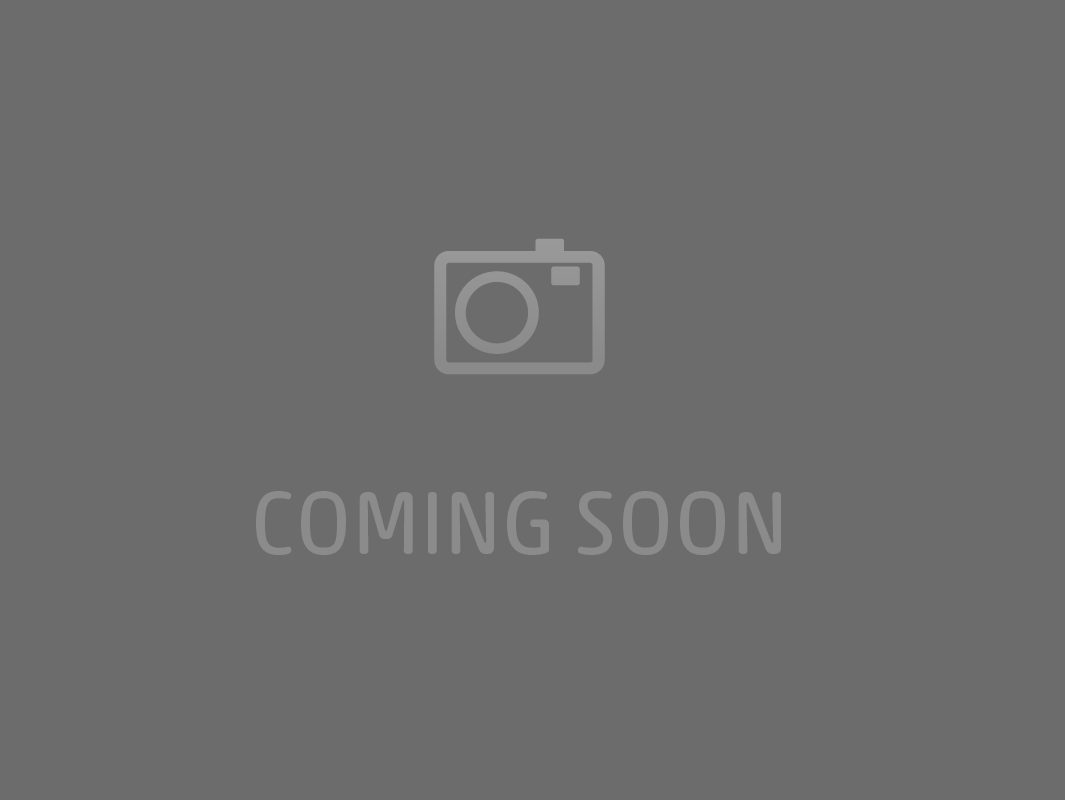}
}
 \subcaptionbox{\CORR{optional}Discretized representation of the data.\label{fig:dataformat}}{
  \centering
\includegraphics[width=0.3\textwidth, height=0.33\textwidth]{images/placeholder1.png}}
\end{figure}

As the policy network is agnostic of the individual player identities, we grouped the input data for each possession into 4 separate channels: the ball, the tracked player, his teammates and the opposing team. At train-time, the input sequences are given to the model as a 5d-tensor in the format $(batch, timestep, entity, x, y)$.

\tb{Micro-action labels.} We extracted micro-goal labels by computing the cell velocity of the discretized input tracking data. We used a velocity grid of $17\times 17$ cells, corresponding to velocities in the range of $(-1,1)$ feet per 1/25s in both directions.  Velocities outside this range were clipped, which applied to <1\% of all frames.

\tb{Macro-goal labels.} To extract macro-goals, we used a heuristic segmentation of the player tracks, where each segment is bounded by periods of relative stationary behavior, as illustrated in figure \ref{fig:tracks}. We used a threshold of 0.25 ft per 1/25s to determine these stationary points. 

To define macro-goals we used a coarse clustering with $10\times 9$ cells of size $5\times 5$ of the left basketball court. The macro-goals were then defined as the cluster in which the player was located during the stationary periods. We used a clustering of $10\times 9$ boxes of $5\times5$ft of the basketball court and additionally imposed a minimal segment length of 15 frames. The final macro-goal is always the final position of the track in the possession.

\tb{Straight-line micro-action labels.} We also extracted the straight-line velocities between the player location $s_t$ and the macro-goal $g_t$. The magnitude of the velocity was chosen randomly between 1 and 7 unit cells, with the direction fixed by $s_t$ and $g_t$. We used these weak labels to pre-train the attention mechanism $m$ on the micro-action output. For the masks, we used the same $17\times17$ velocity grid definition as for the micro-action labels.

\tb{Training procedure.}

Since our input data is extremely sparse in the occupancy representation, to make training feasible we upsampled the input to multiple resolutions by applying max-pooling layers after the input.

During all stages, we used RMSprop with momentum and a batch-size of 16. 
We performed a search over training hyperparameters and found that a learning-rate of $10^{-3}$ (pre-training), $10^{-5}$ (fine-tuning), decay rate $10^{-6}$ and momentum-parameter 0.9 gave good results.  

\tb{Regularization.} To improve the robustness of the policy rollouts we distorted the input tracks with uniform random translations of <8 unit cells, used $L_2$-regularization on the attention masks $m$ and micro-actions $a$, and injected Gaussian noise with $\sigma=10^{-3}$ after the convolutional layers. 
Moreover, we used batch-normalization \cite{ioffe_batch_2015} and gradient clipping to stabilize training.

\subsection{Rollout tracks.}\label{supp:rollout}

\tb{Memory-cell burn-in.}
Our weak macro-goal labels were relatively stationary, however, as the memory cell state is randomly initialized at the start of every sequence prediction, at the beginning of the sequence the memory cell has lower accuracy in its macro-goal prediction. This implies that the macro-planner generally predicts the correct macro-goal only after a certain burn-in time, which imposes a natural ceiling on the predictive accuracy of the macro-planner. For our rollout experiments, we used a burn-in period of 20 frames, and empirically verified that with shorter burn-in periods, the quality of the rollout decreases. \CORR{Put in main text?}  

We also experimented with preserving the memory state between rollouts, but found this did not make a significant difference in the quality of the on-policy rollout evaluations.

\subsection{User study}\label{supp:userstudy}

\begin{figure}[t]
\centering
\includegraphics[width=\textwidth]{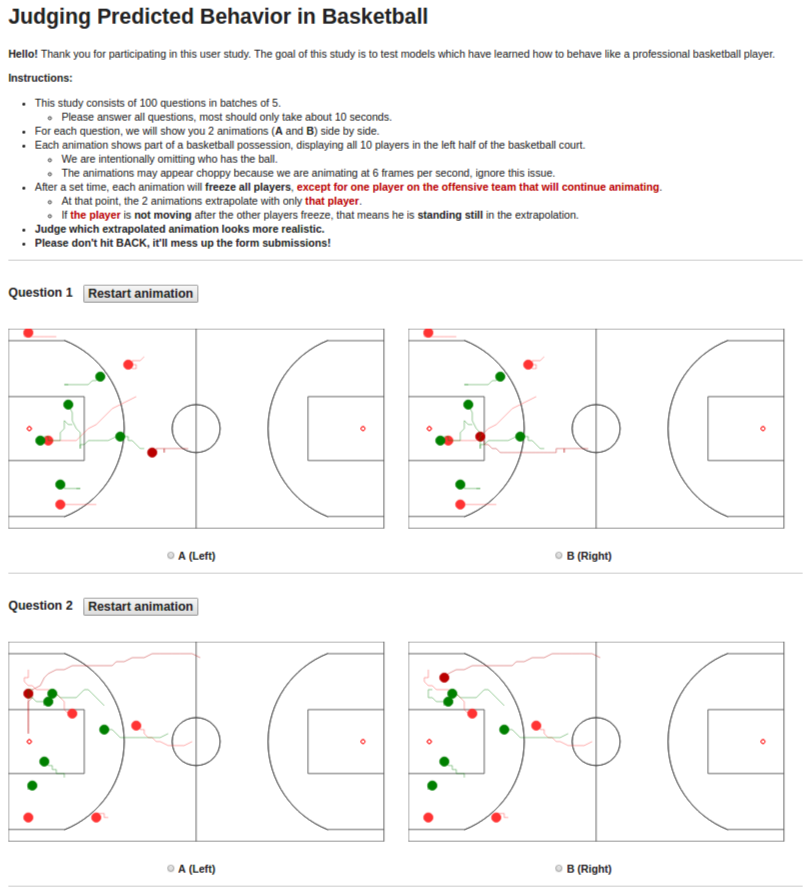}
\caption{User study interface.}
\label{fig:dataformat}
\end{figure}

\tb{Setup.}
To test whether our model produces realistic basketball play behavior, we performed a small-scale user study with domain experts. In the study, the subjects were presented with a set of possessions and rollouts. 

For each possession, the ground truth movements of all players were shown for some time $T_0 > 0$. After $T_0$, a single player continued to move, while the other players were frozen. 
The subjects were presented with two alternatives for the continuation of the player's movement: one generated by a rollout of the hierarchical policy network, the other either by 1) a baseline or 2) the ground truth. The subjects were then asked to indicate which alternative looked more realistic. 

We used a pool of 10 domain experts and 25 possessions as our test data. Each expert was presented with 100 test cases, consisting of 4 pair-wise comparisons of the hierarchical policy network with one of the 3 baselines or the ground truth.

% If comparing against ground truth, for perfectly natural rollout behavior of the hierarchical policy network the subjects would need to pick the hierarchical policy rollout with >50\% probability. 

% \subsection{Attention masks.}\label{supp:attention}

% \subsection{Low-level inspection}
% \subsubsection{Conv layer behavior}
% \subsubsection{Memory cell behavior}

% \INST{Optional?}

% \begin{figure}[H]
% \centering
% \includegraphics[width=0.25\textwidth]{images/placeholder1.png}
% \includegraphics[width=0.25\textwidth]{images/placeholder1.png}
% \caption{}
% \label{fig:memory}
% \end{figure}
